# Supplementary material for: Auto-Gait: Automatic Ataxia Risk Assessment with Computer Vision on Gait Task Videos
Source: arXiv:2203.08215 source file (2022-04-15)
Supplement: Supplementary file 1 [file appendix_multi_class.tex]

\section{Multi-class prediction}

\begin{table}[]
\caption{Ataxia severity prediction  (4 classes: 0, 1, 2, \textgreater{}2) model performance. The training method used here is similar to the one used to generate the results in Table \ref{tab:rist-prediction}}
\label{tab:severity-prediction}
\begin{tabular}{|l|rr|rr|}
\hline
\multicolumn{1}{|c|}{Test} & \multicolumn{2}{l|}{F1 score (\%)}	& \multicolumn{2}{l|}{Accuracy (\%)}	\\ \cline{2-5} 
\multicolumn{1}{|c|}{}	& \multicolumn{1}{c|}{Mean}  & \multicolumn{1}{c|}{STD} & \multicolumn{1}{c|}{Mean}  & \multicolumn{1}{c|}{STD} \\ \hline
10-fold CV	& \multicolumn{1}{r|}{48.17} & 8.76	& \multicolumn{1}{r|}{62.83} & 11.55	\\ \hline
Site 2	& \multicolumn{1}{r|}{32.32} & 6.89	& \multicolumn{1}{r|}{60.89} & 2.64	\\ \hline
Site 3	& \multicolumn{1}{r|}{36.66} & 3.05	& \multicolumn{1}{r|}{69.21} & 5.83	\\ \hline
Site 4	& \multicolumn{1}{r|}{27.17} & 3.93	& \multicolumn{1}{r|}{48.57} & 8.33	\\ \hline
Site 5	& \multicolumn{1}{r|}{65.46} & 14.25	& \multicolumn{1}{r|}{66.43} & 14.48	\\ \hline
Site 6	& \multicolumn{1}{r|}{41.90} & 6.67	& \multicolumn{1}{r|}{60.00} & 8.16	\\ \hline
\end{tabular}
\end{table}
